# Supplementary material for: Massively Parallel Algorithms for Small Subgraph Counting
Source: arXiv:2002.08299 source file (2022-07-18)
Supplement: Supplementary file 3 [file 600-estimation_appendix.tex]

\section{Proofs Missing from Section~\ref	{sec:approx-triangle-counting}}\label{sec:approx-appendix}

\subsection{Approximate Triangle Counting: Bounding the number of Messages Sent/Received by a Machine}
\label{sec:approximate_triangle_counting_bounding_messages}

This section analyzes the estimation algorithm from \cref{sec:approx-triangle-counting}.
Recall, from \cref{sec:computing_the_induced_subgraph}, that we use a $k$-wise independent hash function,
to compute the induced sub-graphs $G[V_i]$, where $k=6\log n$.
