# Supplementary material for: Massively Parallel Algorithms for Small Subgraph Counting
Source: arXiv:2002.08299 source file (2022-07-18)
Supplement: Supplementary file 4 [file 650-estimation_triangle_concentration_appendix.tex]

\subsection{Approximate Triangle Counting: Showing that the Estimate Concentrates}
\label{sec:approximate_triangle_counting_concentration}
